# Supplementary material for: Beating the thermal limit of qubit initialization with a Bayesian Maxwell's demon
Source: arXiv:2110.02046 source file (2022-11-01)
Supplement: Supplementary file 1 [file supplementary.tex]

\section{Discussion on electron temperature}
This initialization method is similar in principle to the famed Maxwell's demon, however instead of explicitly preventing the motion of an electron as the demon would, we simply pre-filter all of the events in which the electron \emph{did} move. 
We now present this technique as a novel cooling method. At the read position, the electron can shuttle to and from a \gls{set}, which acts as our Fermi reservoir. 
Independent measurements show the temperature of this reservoir to be $T_\textrm{e} \approx \SI{260}{\milli\kelvin}$, hence the expected electron spin populations when loading the donor from the reservoir are $P_\uparrow = 1 - P_\downarrow \approx 2.5 \%$.

An alternative metric for the effective temperature that the donor-bound electron sees can be extracted from the tunnel rates to the Fermi reservoir. 
Applying Fermi's golden rule, we take the tunnel rate of a spin-up electron to the reservoir to be
\begin{equation}
    \Gamma_{D^0_\uparrow \rightarrow D^+} = \dfrac{2\pi}{\hbar} \left|\bra{D^0_\uparrow} H' \ket{D^+}\right|^2 \rho(E_\uparrow)
\end{equation}
where $\bra{D^0_\uparrow} H' \ket{D^+}$ is the transition matrix element arising from device specific arrangements and $\rho(E_\uparrow)$ is the density of free states in the reservoir at the Zeeman energy $E_\uparrow \approx \SI{82.5}{\micro\electronvolt}$. 
Similarly, the tunnel rate of a spin-down electron to the reservoir is $\Gamma_{D^0_\downarrow \rightarrow D^+} = \dfrac{2\pi}{\hbar} \left|\bra{D^0_\downarrow} H' \ket{D^+}\right|^2 \rho(E_\downarrow)$.
Here, the donor state is described by its charge degree of freedom, i.e. the presence or absence of an electron, with $D^0$ indicating a neutrally charged donor, and $D^+$ being a positively charged donor.
Therefore, the electron spin subscript only applies to the neutral donor $D^0_{\uparrow, \downarrow}$.
We claim that the transition matrix elements for each electron spin state are identical (i.e. $\left|\bra{D^0_\uparrow} H' \ket{D^+}\right|^2 = \left|\bra{D^0_\downarrow} H' \ket{D^+}\right|^2$), as the nature of the potential landscape is identical for each spin state, and the \gls{set} reservoir has equal parts spin-up and spin-down unoccupied states across all energies. 
Thus, we define a quantity
\begin{equation}
    R = \dfrac{\Gamma_{D^0_\uparrow \rightarrow D^+}}{\Gamma_{D^0_\downarrow \rightarrow D^+}} = \dfrac{\rho(E_\uparrow)}{\rho(E_\downarrow)}
\end{equation}
to explore the effect of temperature on electron spin readout contrast.
Assuming the \gls{set} reservoir follows a Fermi distribution
\setlength{\jot}{15pt} % Slightly more space between lines with large fractions
\begin{align}
    R &= \dfrac{1 - \dfrac{1}{1 + \exp(E_\uparrow/k_B T)}}
               {1 - \dfrac{1}{1 + \exp(E_\downarrow/k_B T)}} \\
    &= \dfrac{\exp(E_\uparrow/k_B T)}{\exp(E_\uparrow/k_B T) + 1} \cdot 
         \dfrac{\exp(E_\downarrow/k_B T) + 1}{\exp(E_\downarrow/k_B T)}. \\
\intertext{Next, let $E_{\uparrow, \downarrow} = E_f \pm \Delta E/2$ with $E_f = 0$ for simplicity}
    &= \exp(\Delta E / k_B T) \dfrac{1 + \exp(-\Delta E / 2 k_B T)}
                                    {1 + \exp(\Delta E / 2 k_B T)}
\end{align}
where the spin state energies are tuned about the Fermi level, $E_f$, and  Zeeman split $\Delta E = \gamma_\textrm{e} B_0$. 
For a vanishing energy splitting between spin eigenstates, or equivalently an infinite temperature, $\lim\limits_{\Delta E \rightarrow 0} R = 1$. For large energy splitting, $\Delta E \gg k_B T$, we recover $R \sim \exp(\Delta E / k_B T)$. We now use the ratio $R(\Delta E, T)$ as a tool to probe the reservoir temperature as seen by the donor-bound electron.

% \begin{figure*}
%     \centering
%     \includegraphics{plots/temperature-white.png}
%     \caption{}
%     \label{fig:R_temperature}
% \end{figure*}

% Look at Figure \ref{fig:R_temperature}

\begin{figure}[htbp]
    \centering
    \includegraphics[width=\columnwidth]{plots/max_contrast_temperature_white.png}
    \caption{This shows the electron readout contrast for an electron with fixed electrochemical potential and spin splitting (here $E_Z \approx \gamma_e B_0 = \SI{165}{\micro\electronvolt}$) coupled to a Fermi reservoir at temperature $T_{\textrm{e}}$. 
    The spin contrast is shown as a function of readout time, and the maximum contrast in time is plotted on the lower axis. 
    The curve indicates that below $T_{\textrm{e}} \approx \SI{100}{\milli\kelvin}$ the expected spin contrast is $\sim$100 \%. 
    The contrast is analytically determined to be $C = \exp(-t/\tau_{\downarrow, \textrm{out}}) - \exp(-t/\tau_{\uparrow, \textrm{out}})$.
    }
    \label{fig:max_contrast}
\end{figure}

We can also determine the expected spin readout contrast ($\mu_\uparrow - \mu_\downarrow$) by
